# Supplementary material for: Predictive Whole-Body Control of Humanoid Robot Locomotion
Source: arXiv:2004.07699 source file (2020-04-16)
Supplement: Supplementary file 1 [file appendix.tex]

%!TEX root = ../steprecovery.tex
% \appendix
